# Supplementary material for: Jointly Optimizing Debiased CTR and Uplift for Coupons Marketing: A Unified Causal Framework
Source: arXiv:2602.12972 source file (2026-09-08)
Supplement: Supplementary file 1 [file appendix.tex]

\appendix

\section{Theoretical Analysis}\label{appendix_proof}

\subsection{Proof of Theorem \ref{Convergence of Unit Uplift}}

We aim to show that minimizing the counterfactual regularization loss $\mathcal{L}_{\text{x-base}}$ and $\mathcal{L}_{\text{x-treat}}$ guarantees the convergence of the estimated unit uplift $\hat{\eta}$ to the true structural uplift $\eta$. 
% Without loss of generality, we focus on the control group reconstruction (base regularization); the proof for the treated group follows symmetrically.
\subsubsection{Proof of Convergence for $\mathcal{L}_{\text{x-treat}}$}

\begin{proof}
We now demonstrate that minimizing the counterfactual regularization loss for the treated group, $\mathcal{L}_{\text{x-treat}}$, similarly guarantees the identification of the unit uplift.

Let $\mathcal{L}_{\text{x-treat}}$ denote the discrepancy between the estimated counterfactual treated outcome $\hat{p}'_t(\mathbf{x}_i, t_i)$ and the true observed treated outcome $p_t(\mathbf{x}_i, t_i)$.

The estimated counterfactual treated outcome is derived by adding the estimated treatment effect to the predicted baseline:

\begin{align}
\hat{p}'_t(\mathbf{x}_i, \hat{t}_i) = \hat{p}_0(\mathbf{x}_i) + \hat{\eta}_i \cdot \hat{t}_i.
\end{align}

The true structural relationship between the treated and baseline outcomes is given by:

\begin{align}
p_t(\mathbf{x}_i, t_i) = p_0(\mathbf{x}_i) + \eta_i \cdot t_i.
\end{align}

We define the error term $\Delta_i$ as the absolute difference between the estimated and true treated outcome:

\begin{align}
\Delta_i &= | \hat{p}'_t(\mathbf{x}_i, \hat{t}_i) - p_t(\mathbf{x}_i, t_i) | \nonumber \\
&= | (\hat{p}_0(\mathbf{x}_i) + \hat{\eta}_i \hat{t}_i) - (p_0(\mathbf{x}_i) + \eta_i t_i) |.
\end{align}

To isolate the uplift error term $(\hat{\eta}_i - \eta_i)$, we rearrange the terms and introduce the cross-term $\hat{\eta}_i t_i - \hat{\eta}_i t_i = 0$:

\begin{align}
\Delta_i &= | (\hat{p}_0(\mathbf{x}_i) - p_0(\mathbf{x}_i)) + (\hat{\eta}_i \hat{t}_i - \eta_i t_i) | \nonumber \\
&= | (\hat{p}_0 - p_0) + (\hat{\eta}_i \hat{t}_i - \hat{\eta}_i t_i + \hat{\eta}_i t_i - \eta_i t_i) | \nonumber \\
&= | \underbrace{(\hat{p}_0 - p_0)}_{\text{Base Error}} + \underbrace{\hat{\eta}_i (\hat{t}i - t_i)}_{\text{Intensity Error}} + \underbrace{t_i (\hat{\eta}_i - \eta_i)}_{\text{Uplift Error}} |.
\end{align}

By the Triangle Inequality ($|a + b| \le |a| + |b|$), we bound the error magnitude:
\begin{align}
\Delta_i \le | \hat{p}_0 - p_0 | + | \hat{\eta}_i | \cdot | \hat{t}_i - t_i | + | t_i | \cdot | \hat{\eta}_i - \eta_i |.
\end{align}


By assumption \ref{intensity}, the true treatment intensity is bounded away from zero ($|t_i| \ge t_{min} > 0$). Therefore, the factor $|t_i|$ is strictly positive. For the product to vanish, it must be that the uplift error vanishes:

\begin{align}
| \hat{\eta}_i - \eta_i | \xrightarrow{p} 0.
\end{align}

This confirms that minimizing the counterfactual regularization loss on the treated group also guarantees that the estimated unit uplift $\hat{\eta}_i$ converges in probability to the true structural uplift $\eta_i$.
\end{proof}


\subsubsection{Proof of Convergence for $\mathcal{L}_{\text{x-base}}$}
\begin{proof}
Let $\mathcal{L}_{\text{x-base}}$ denote the discrepancy between the estimated counterfactual baseline $\hat{p}'_0(\mathbf{x}_i)$ and the true observed baseline $p_0(\mathbf{x}_i)$.

The estimated counterfactual baseline is derived by subtracting the estimated treatment effect from the predicted treated outcome:


\begin{align}
\hat{p}'_0(\mathbf{x}_i) = \hat{p}_t(\mathbf{x}_i, \hat{t}_i) - \hat{\eta}_i \cdot \hat{t}_i.
\end{align}

The true structural relationship between the baseline and treated outcomes is given by:
\begin{align}
p_0(\mathbf{x}_i) = p_t(\mathbf{x}_i, {t}_i) - \eta_i \cdot t_i.
\end{align}

We define the error term $\Delta_i$ as the absolute difference between the estimated and true baseline:
\begin{align}
\Delta_i &= | \hat{p}'_0(\mathbf{x}_i) - p_0(\mathbf{x}_i) | \nonumber \\
&= | (\hat{p}_t(\mathbf{x}_i, \hat{t}_i) - \hat{\eta}_i \hat{t}_i) - (p_t(\mathbf{x}_i, t_i) - \eta_i t_i) |.
\end{align}

To isolate the uplift error term $(\eta_i - \hat{\eta}_i)$, we rearrange the terms and introduce the cross-term $\eta_i \hat{t}_i - \eta_i \hat{t}_i = 0$:

\begin{align}
\Delta_i &= | (\hat{p}_t(\mathbf{x}_i, \hat{t}_i) - p_t(\mathbf{x}_i, t_i)) + (\eta_i t_i - \hat{\eta}_i \hat{t}_i) | \nonumber \\
&= | (\hat{p}_t(\mathbf{x}_i, \hat{t}_i) - p_t(\mathbf{x}_i, t_i)) + (\eta_i t_i - \eta_i \hat{t}_i + \eta_i \hat{t}_i - \hat{\eta}_i \hat{t}_i) | \nonumber \\
&= | \underbrace{(\hat{p}_t(\mathbf{x}_i, \hat{t}_i) - p_t(\mathbf{x}_i, t_i))}_{\text{Outcome Error}} + \underbrace{\eta_i (t_i - \hat{t}_i)}_{\text{intensity Error}} + \underbrace{\hat{t}_i (\eta_i - \hat{\eta}_i)}_{\text{Uplift Error}} |.
\end{align}

By the Triangle Inequality ($|a + b| \le |a| + |b|$), we bound the error magnitude:

\begin{align}
\Delta_i \le | \hat{p}_t(\mathbf{x}_i, \hat{t}_i) - p_t(\mathbf{x}_i, t_i) | + | \eta_i | \cdot | t_i - \hat{t}_i | + | \hat{t}_i | \cdot | \eta_i - \hat{\eta}_i |.
\end{align}

To prove the convergence of $\hat{p}_t(\mathbf{x}_i, \hat{t}_i) - p_t(\mathbf{x}_i, t_i)$ term, we apply the triangle inequality to decompose the error term into two components: the estimation error of the density model and the approximation error caused by the treatment perturbation.
\begin{align}
\left| \hat{p}_t(\mathbf{x}_i, \hat{t}_i) - p_t(\mathbf{x}_i, t_i) \right| &= \left| \hat{p}_t(\mathbf{x}_i, \hat{t}_i) - p_t(\mathbf{x}_i, \hat{t}_i) + p_t(\mathbf{x}_i, \hat{t}_i) - p_t(\mathbf{x}_i, t_i) \right| \nonumber\\
&\le {\left| \hat{p}_t(\mathbf{x}_i, \hat{t}_i) - p_t(\mathbf{x}_i, \hat{t}_i) \right|} + {\left| p_t(\mathbf{x}_i, \hat{t}_i) - p_t(\mathbf{x}_i, t_i) \right|} 
\end{align}

Based on Assumption \ref{estimators}, as the model training converges (sample size $N \to \infty$), the estimator $\hat{p}_t$ approaches $p_t$ uniformly over the domain. Therefore, for any input $(\mathbf{x}_i, \hat{t}_i)$, we have:
\begin{align}
\lim_{N \to \infty} \left| \hat{p}_t(\mathbf{x}_i, \hat{t}_i) - p_t(\mathbf{x}_i, \hat{t}_i) \right| = 0
\end{align}

Based on Assumption \ref{intensity}, we can bound the perturbation error by the distance between the estimated treatment $\hat{t}_i$ and the true treatment $t_i$:$$\left| p_t(\mathbf{x}_i, \hat{t}_i) - p_t(\mathbf{x}_i, t_i) \right| \le L_p \| \hat{t}_i - t_i \|_2$$Since it is given that the treatment estimation (e.g., via LHUC GateNet) converges, i.e., $\| \hat{t}_i - t_i \|_2 \to 0$, it follows that:
\begin{align}
\lim_{\| \hat{t}_i - t_i \| \to 0} \left| p_t(\mathbf{x}_i, \hat{t}_i) - p_t(\mathbf{x}_i, t_i) \right| = 0
\end{align}

Therefore, we conclude that:
\begin{align}
\left| \hat{p}_t(\mathbf{x}_i, \hat{t}_i) - p_t(\mathbf{x}_i, t_i) \right| \to 0
\end{align}

By assumption\ref{intensity}, the true intensity is bounded away from zero ($|t_i| \ge \epsilon > 0$). Since $\hat{t}_i$ is consistent ($\hat{t}_i \to t_i$), it follows that for sufficiently large $N$, $|\hat{t}_i|$ is also bounded away from zero.
Therefore, the only solution for the product to vanish is for the uplift error to vanish:

\begin{align}
| \eta_i - \hat{\eta}_i | \xrightarrow{p} 0.
\end{align}

This concludes the proof that the estimated unit uplift $\hat{\eta}_i$ converges in probability to the true structural uplift $\eta_i$.



\end{proof}




\section{Experiment Details}

\subsection{Implementation Details}
\begin{figure}[H]
  \centering
  \includegraphics[width=\linewidth]{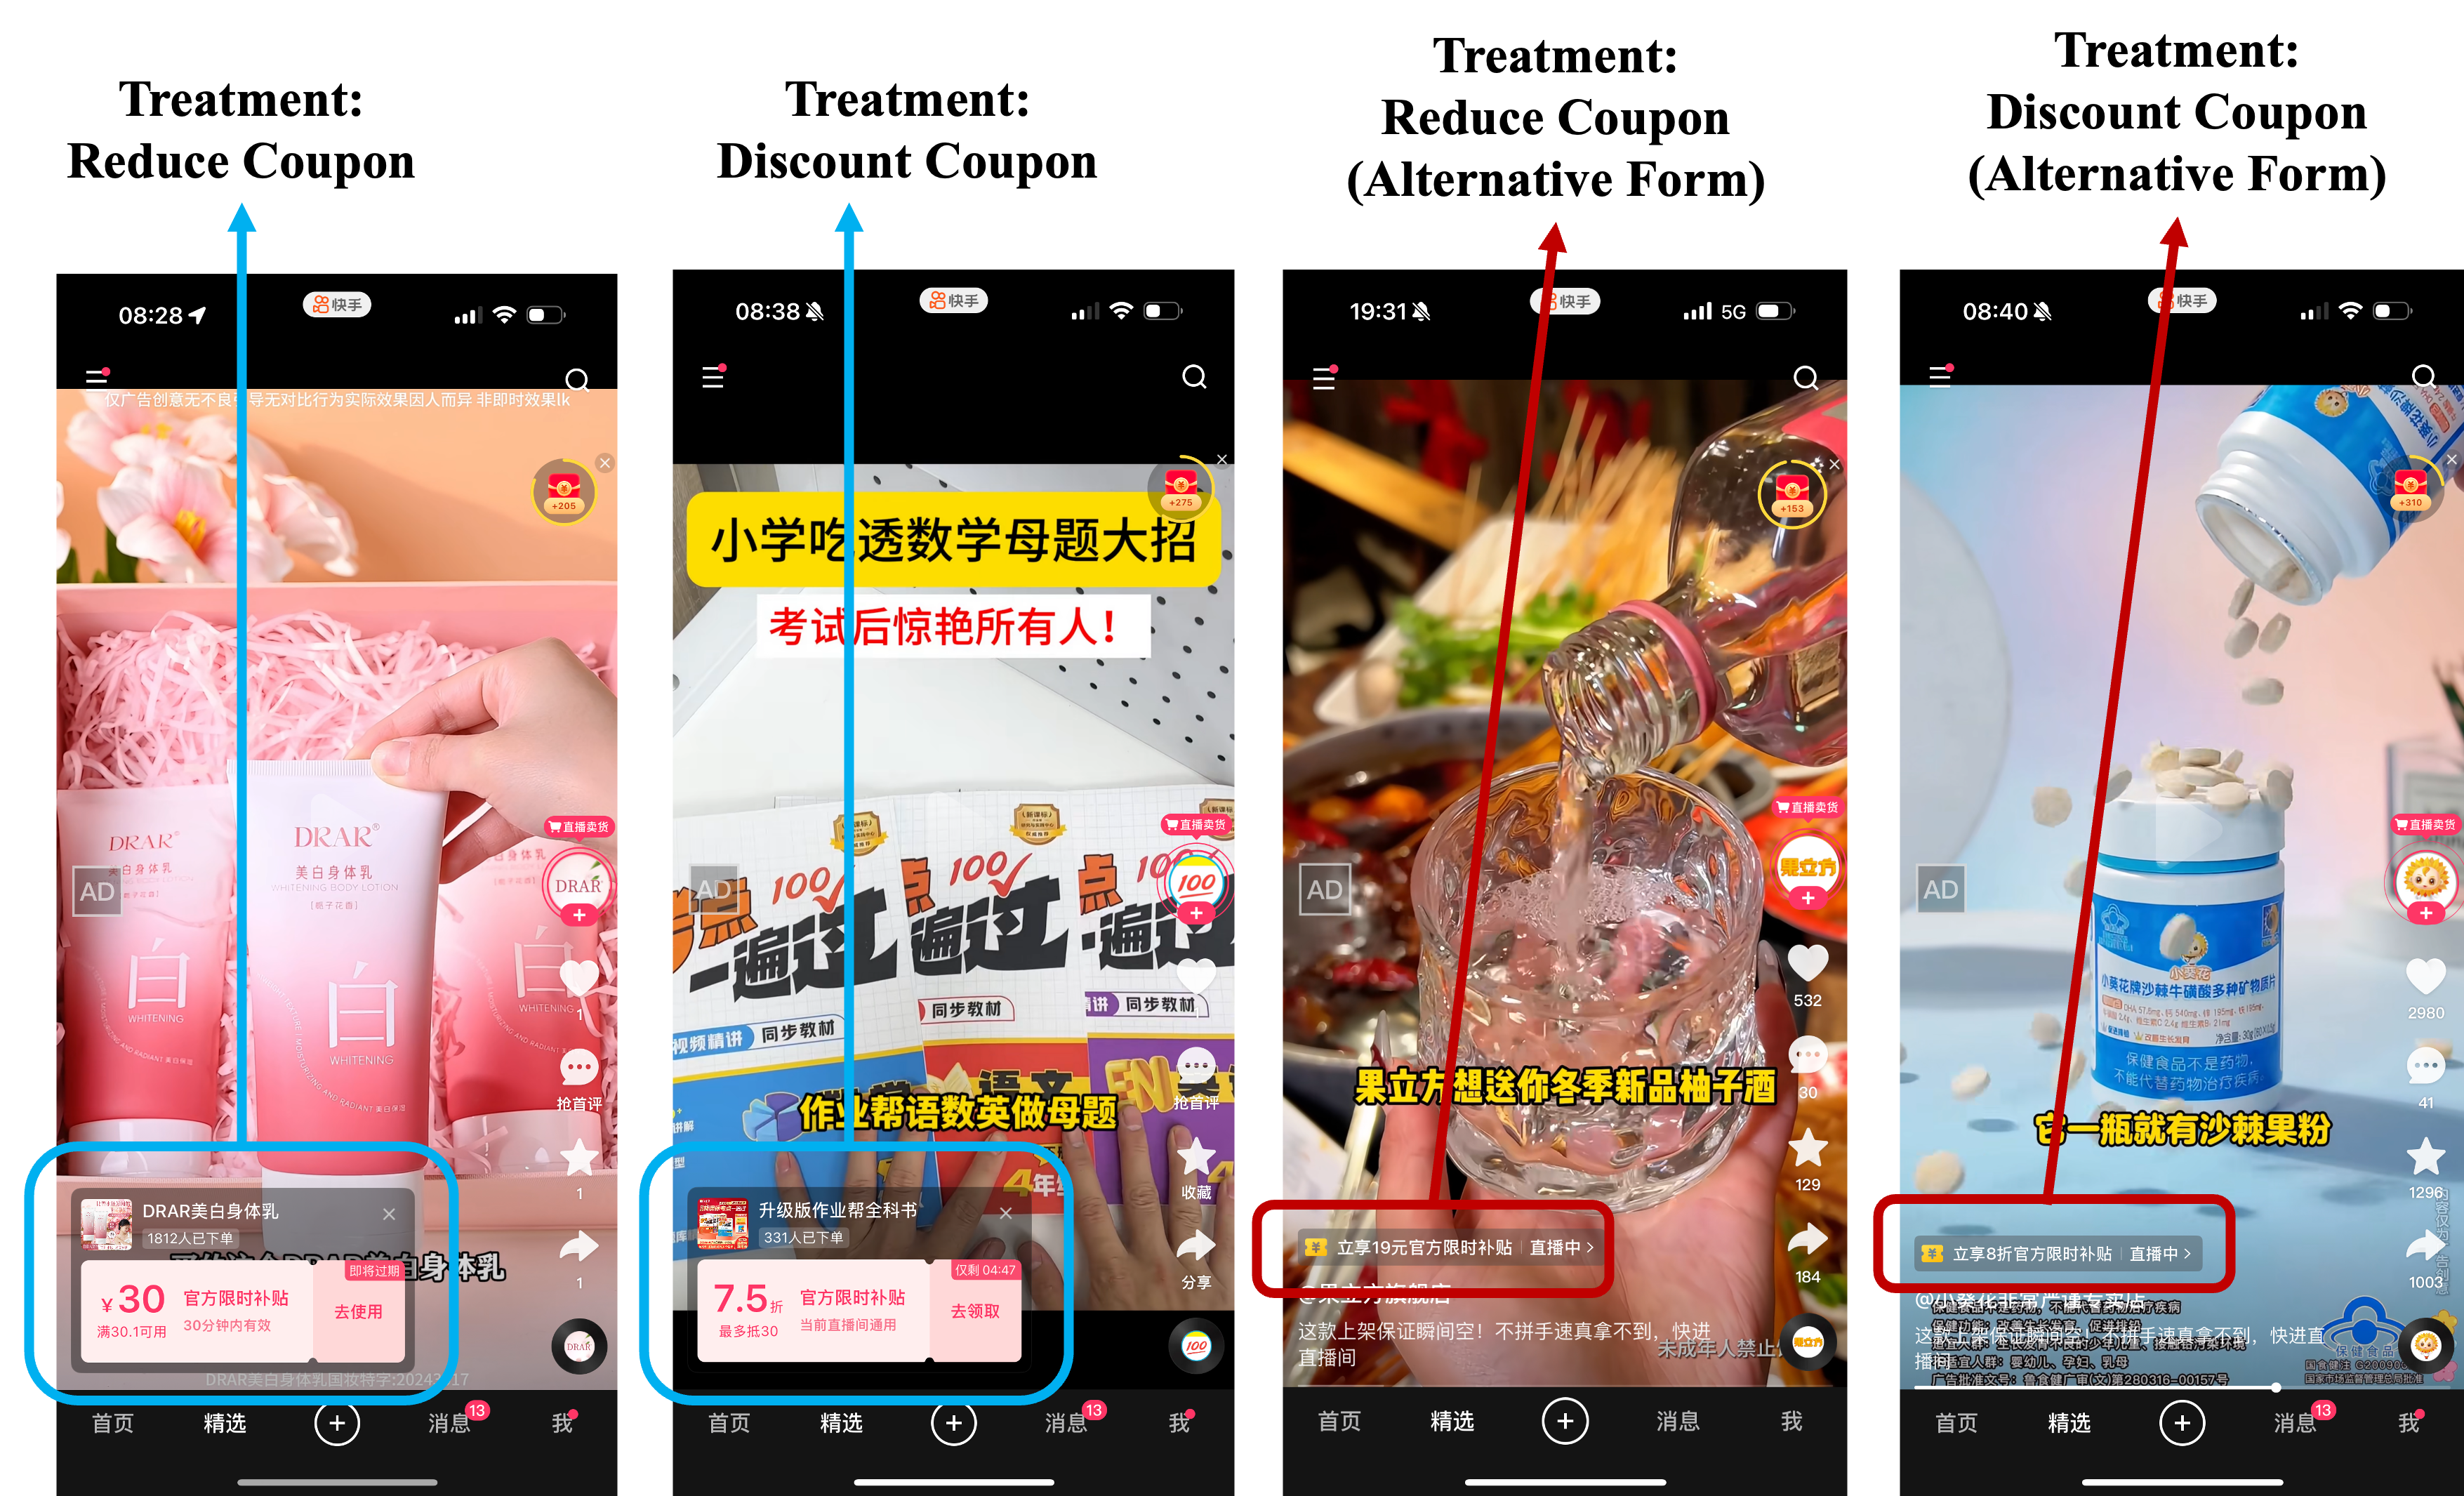}
  \caption{The illustration of coupon scenario. These pre-click promotional details can significantly influence user click-through rates.}
  \label{fig:scenario}
\end{figure}

The scenario is illustrated in Figure \ref{fig:scenario}.
Marketing in this scenario launches different coupon campaigns for different customer segments to motivate more users to click and complete purchases on the platform. 
The treatments are promoted to some group of users once user shows interest in specific items or categories. 
Interventions include multiple coupon styles (e.g., full-reduction coupons, percentage discount coupons) and denominations (e.g., 0.7x, 0.9x discounts). Coupons are surfaced in the lower area of the screen to attract user attention and increase overall click-through rate (CTR). The delivery policy follows a greedy strategy that assigns a coupon to users with the highest expected net gain, defined as predicted revenue lift minus coupon cost. 
